# Supplementary material for: Efficient Vision-based Vehicle Speed Estimation
Source: arXiv:2505.01203 source file (2025-05-02)
Supplement: Supplementary file 2 [file appendix_old.tex]

\appendix
% \section{Experiments results}\label{chap:app_a}

\begin{table*}[]
\resizebox{\linewidth}{!}{
\begin{tabular}{lcccccc}
Model &
  \begin{tabular}[c]{@{}c@{}}Input size \\ (px)\end{tabular} &
  \begin{tabular}[c]{@{}c@{}}Mean error \\ (km/h)\end{tabular} &
  \begin{tabular}[c]{@{}c@{}}Median error \\ (km/h)\end{tabular} &
  \begin{tabular}[c]{@{}c@{}}95-th percentile \\ (km/h)\end{tabular} &
  \begin{tabular}[c]{@{}c@{}}Mean precision \\ (\%)\end{tabular} &
  \begin{tabular}[c]{@{}c@{}}Mean recall \\ (\%)\end{tabular} \\ \hline
\multirow{3}{*}{Nano}          & 480 x 270 & 0.87          & 0.70          & 2.09          & 88.08          & 91.23           \\
                               & 640 x 360 & 0.80          & 0.64          & 2.04          & 89.69          & 92.25           \\
                               & 960 x 540 & 0.85          & 0.66          & 2.17          & 90.60          & \textbf{92.74}  \\ \hline
\multirow{3}{*}{Nano distill}  & 480 x 270 & 0.98          & 0.73          & 2.09          & 88.08          & 91.23           \\
                               & 640 x 360 & 0.90          & 0.73          & 2.24          & 86.00          & 89.30           \\
                               & 960 x 540 & 0.87          & 0.70          & 2.19          & 84.73          & 86.92           \\ \hline
\multirow{3}{*}{Small}         & 480 x 270 & 0.87          & 0.68          & 2.16          & 91.08          & 91.85           \\
                               & 640 x 360 & \textbf{0.76} & \textbf{0.58} & \textbf{2.01} & 91.02          & 92.16           \\
                               & 960 x 540 & 0.81          & 0.62          & 2.08          & \textbf{92.09} & 91.86           \\ \hline
\multirow{3}{*}{Small distill} & 480 x 270 & 0.91          & 0.73          & 2.24          & 85.45          & 91.00           \\
                               & 640 x 360 & 0.84          & 0.65          & 2.16          & 85.05          & 89.68           \\
                               & 960 x 540 & 0.83          & 0.70          & 2.16          & 84.73          & 90.07           \\ \hline
\multirow{3}{*}{Medium}        & 480 x 270 & 0.84          & 0.67          & 2.15          & 91.55          & 87.44           \\
                               & 640 x 360 & 0.86          & 0.69          & 2.21          & 91.32          & 90.68           \\
                               & 960 x 540 & 0.82          & 0.63          & 2.13          & 91.23          & 91.01           \\ \hline
\multirow{3}{*}{Large}         & 480 x 270 & 0.87          & 0.70          & 2.25          & 90.85          & 91.12           \\
                               & 640 x 360 & 0.84          & 0.66          & 2.16          & 90.34          & 90.67           \\
                               & 960 x 540 & 0.81          & 0.62          & 2.14          & 91.11          & 89.61           \\ \hline
\end{tabular}}
\caption{Speed measurement evaluation on BrnoCompSpeed split test C, using FP16.}
\label{tb:fp16titan}
\end{table*}

\begin{figure}[h]
    \centering
    \includegraphics[width=1\columnwidth]{images/graph.pdf}
    \caption{Comparison of median speed measurement and performance for different model and input sizes in FP16 mode on Titan V.}
    \label{img:chart_nano}
\end{figure}

\begin{figure}[h]
    \centering
    \includegraphics[width=1\columnwidth]{images/arrowsbest.pdf}
    \caption{Quantization increases performance of all model configurations without a loss in median speed estimation accuracy, graph contains data for Titan V in $640 \times 360$ input resolution. }
    \label{img:chart_nano}
\end{figure}


\begin{comment}
%\begin{landscape}
\centering
\begin{table*}[h]
\begin{tabular}{cccccccc}
\hline
Models &
  \begin{tabular}[c]{@{}c@{}}Input size \\ (px)\end{tabular} &
  \begin{tabular}[c]{@{}c@{}}Mean error \\ (km/h)\end{tabular} &
  \begin{tabular}[c]{@{}c@{}}Median error \\ (km/h)\end{tabular} &
  \begin{tabular}[c]{@{}c@{}}95-th percentile \\ (km/h)\end{tabular} &
  \begin{tabular}[c]{@{}c@{}}Mean precision \\ (\%)\end{tabular} &
  \begin{tabular}[c]{@{}c@{}}Mean recall \\ (\%)\end{tabular} &
  FPS \\ \hline
\multirow{3}{*}{Nano}          & 480 x 270 & 0.86          & 0.69          & 2.10          & 88.05          & 91.20          & 295          \\
                               & 640 x 360 & \textbf{0.80} & 0.64          & 2.04          & 89.62          & 91.36          & 224          \\
                               & 960 x 540 & 0.82          & 0.66          & 2.11          & 91.24          & 89.97          & 148          \\ \hline
\multirow{3}{*}{Nano distill}  & 480 x 270 & 0.98          & 0.74          & 2.46          & 81.64          & 88.14          & \textbf{296} \\
                               & 640 x 360 & 0.90          & 0.81          & 2.24          & 85.94          & 88.44          & 227          \\
                               & 960 x 540 & 0.87          & 0.70          & 2.19          & 84.67          & 86.09          & 145          \\ \hline
\multirow{3}{*}{Small}         & 480 x 270 & 0.87          & 0.68          & 0.69          & 91.03          & \textbf{92.11} & 229          \\
                               & 640 x 360 & 0.81          & \textbf{0.58} & \textbf{2.01} & 91.02          & 91.87          & 142          \\
                               & 960 x 540 & 0.81          & 0.63          & 2.07          & \textbf{92.15} & 90.99          & 95           \\ \hline
\multirow{3}{*}{Small distill} & 480 x 270 & 0.91          & 0.73          & 2.23          & 85.38          & 91.93          & 226          \\
                               & 640 x 360 & 0.84          & 0.65          & 2.15          & 85.07          & 88.85          & 143          \\
                               & 960 x 540 & 0.86          & 0.67          & 2.15          & 84.79          & 89.24          & 93           \\ \hline
\multirow{3}{*}{Medium}        & 480 x 270 & 0.84          & 0.67          & 2.23          & 91.49          & 91.93          & 187          \\
                               & 640 x 360 & 0.86          & 0.69          & 2.19          & 91.31          & 89.76          & 128          \\
                               & 960 x 540 & 0.83          & 0.66          & 2.14          & 90.95          & 90.13          & 55           \\ \hline
\multirow{3}{*}{Large}         & 480 x 270 & 0.87          & 0.70          & 2.23          & 90.78          & 90.34          & 130          \\
                               & 640 x 360 & 0.84          & 0.66          & 2.15          & 90.29          & 89.75          & 95           \\
                               & 960 x 540 & 0.82          & 0.67          & 2.10          & 91.15          & 90.93          & 40           \\ \hline
\end{tabular}
\caption{Speed measurement evaluation on BrnoCompSpeed split test C, using FP32 and running on NVIDIA RTX 2080.}
\label{tb:fp32rtx}
\end{table*}
%\end{landscape}
\end{comment}


%\begin{landscape}
\begin{table*}[h]
\centering
\begin{tabular}{ccccccc}g
\hline
Models &
  \begin{tabular}[c]{@{}c@{}}Input size\\ (px)\end{tabular} &
  \begin{tabular}[c]{@{}c@{}}Mean error \\ (km/h)\end{tabular} &
  \begin{tabular}[c]{@{}c@{}}Median error \\ (km/h)\end{tabular} &
  \begin{tabular}[c]{@{}c@{}}95-th percentile \\ (km/h)\end{tabular} &
  \begin{tabular}[c]{@{}c@{}}Mean precision \\ (\%)\end{tabular} &
  \begin{tabular}[c]{@{}c@{}}Mean precision \\ (\%)\end{tabular} \\ \hline
\multirow{3}{*}{Nano}          & 480 x 270 & 0.87          & 0.69          & 2.09          & 88.08          & 91.23           \\
                               & 640 x 360 & \textbf{0.80} & 0.64          & 2.04          & 89.69          & 92.25           \\
                               & 960 x 540 & 0.82          & 0.66          & 2.17          & 91.15          & 90.10           \\ \hline
\multirow{3}{*}{Nano distill}  & 480 x 270 & 0.98          & 0.74          & 2.47          & 81.71          & 87.39           \\
                               & 640 x 360 & 0.90          & 0.81          & 2.24          & 86.00          & 89.15           \\
                               & 960 x 540 & 0.87          & 0.70          & 2.19          & 84.72          & 86.53           \\ \hline
\multirow{3}{*}{Small}         & 480 x 270 & 0.87          & 0.68          & 2.16          & 91.08          & \textbf{92.85}  \\
                               & 640 x 360 & 0.81          & \textbf{0.58} & \textbf{2.01} & 91.02          & 92.16           \\
                               & 960 x 540 & 0.81          & 0.63          & 2.08          & \textbf{92.11} & 91.14           \\ \hline
\multirow{3}{*}{Small distill} & 480 x 270 & 0.91          & 0.73          & 2.24          & 85.45          & 91.00           \\
                               & 640 x 360 & 0.84          & 0.65          & 2.16          & 85.05          & 89.58           \\
                               & 960 x 540 & 0.86          & 0.67          & 2.16          & 84.73          & 90.07           \\ \hline
\multirow{3}{*}{Medium}        & 480 x 270 & 0.84          & 0.67          & 2.15          & 91.55          & 92.44           \\
                               & 640 x 360 & 0.86          & 0.69          & 2.21          & 91.32          & 90.68           \\
                               & 960 x 540 & 0.83          & 0.66          & 2.14          & 91.10          & 91.00           \\ \hline
\multirow{3}{*}{Large}         & 480 x 270 & 0.87          & 0.70          & 2.25          & 90.85          & 91.12           \\
                               & 640 x 360 & 0.84          & 0.66          & 2.16          & 90.34          & 90.67           \\
                               & 960 x 540 & 0.82          & 0.64          & 2.13          & 91.21          & 90.85           \\ \hline 
\end{tabular}
\caption{Speed measurement evaluation on BrnoCompSpeed split test C, using FP32.}
\label{tb:fp32titan}
\end{table*}
%\end{landscape}

\begin{comment}
%\begin{landscape}
    \begin{table*}[h]
    \centering
    \begin{tabular}{@{}cccccccc@{}}
    \toprule
    Models &
  \begin{tabular}[c]{@{}c@{}}Input size \\ (px)\end{tabular} &
  \begin{tabular}[c]{@{}c@{}}Mean error \\ (km/h)\end{tabular} &
  \begin{tabular}[c]{@{}c@{}}Median error \\ (km/h)\end{tabular} &
  \begin{tabular}[c]{@{}c@{}}95-th percentile \\ (km/h)\end{tabular} &
  \begin{tabular}[c]{@{}c@{}}Mean precision \\ (\%)\end{tabular} &
  \begin{tabular}[c]{@{}c@{}}Mean recall \\ (\%)\end{tabular} &
  FPS \\ \midrule
    \multirow{3}{*}{Nano}          & 480 x 270 & 0.86 & 0.69 & 2.10 & 88.05 & 91.20 &\textbf{436} \\
                                   & 640 x 360 & 0.80 & 0.64 & 2.04 & 89.62 & 91.36 &311 \\
                                   & 960 x 540 & 0.85 & 0.66 & 2.17 & 90.42 & 91.86 &194 \\ \midrule
    \multirow{3}{*}{Nano distill}  & 480 x 270 & 0.98 & 0.74 & 2.46 & 87.64 & 91.51 &360 \\
                                   & 640 x 360 & 0.90 & 0.73 & 2.24 & 85.94 & 88.44 &317 \\
                                   & 960 x 540 & 0.87 & 0.70 & 2.19 & 84.60 & 86.04 &196 \\ \midrule
    \multirow{3}{*}{Small}         & 480 x 270 & 0.87 & 0.68 & 2.15 & 91.03 & 90.11 &252 \\
                                   & 640 x 360 & 0.76 & 0.58 & 2.01 & 91.02 & 91.27 &243 \\
                                   & 960 x 540 & 0.81 & 0.62 & 2.09 & 91.91 & 91.09 &145 \\ \midrule
    \multirow{3}{*}{Small distill} & 480 x 270 & 0.90 & 0.73 & 2.23 & 85.38 & 91.93 &223 \\
                                   & 640 x 360 & 0.84 & 0.65 & 2.15 & 85.07 & 88.85 &244 \\
                                   & 960 x 540 & 0.82 & 0.71 & 2.15 & 84.78 & 89.24 &144 \\ \midrule
    \multirow{3}{*}{Medium}        & 480 x 270 & 0.84 & 0.67 & 2.15 & 91.49 & 86.51 &448 \\
                                   & 640 x 360 & 0.86 & 0.69 & 2.19 & 91.31 & 89.76 &183 \\
                                   & 960 x 540 & 0.81 & 0.63 & 2.14 & 90.92 & 90.13 &110 \\ \midrule
    \multirow{3}{*}{Large}         & 480 x 270 & 0.86 & 0.69 & 2.23 & 90.78 & 90.34 &356 \\
                                   & 640 x 360 & 0.83 & 0.66 & 2.15 & 90.29 & 89.75 &143 \\
                                   & 960 x 540 & 0.81 & 0.64 & 2.10 & 91.14 & 90.93 &90 \\ \bottomrule
    \end{tabular}
    \caption{Speed measurement evaluation on BrnoCompSpeed split test C, using FP16 and running on RTX 2080 GPU.}
    \label{tb:fp16rtx}
    \end{table*}
%\end{landscape}
\end{comment}


%\begin{landscape}
\begin{table*}[]
\begin{tabular}{lcccccc}
\hline
Models &
  \begin{tabular}[c]{@{}c@{}}Input size \\ (px)\end{tabular} &
  \begin{tabular}[c]{@{}c@{}}Mean error \\ (km/h)\end{tabular} &
  \begin{tabular}[c]{@{}c@{}}Median error \\ (km/h)\end{tabular} &
  \begin{tabular}[c]{@{}c@{}}95-th percentile \\ (km/h)\end{tabular} &
  \begin{tabular}[c]{@{}c@{}}Mean precision \\ (\%)\end{tabular} &
  \begin{tabular}[c]{@{}c@{}}Mean recall \\ (\%)\end{tabular} \\ \hline
\multirow{3}{*}{Nano}          & 480 x 270 & 0.87          & 0.70          & 2.09          & 88.08          & 91.23           \\
                               & 640 x 360 & 0.80          & 0.64          & 2.04          & 89.69          & 92.25           \\
                               & 960 x 540 & 0.85          & 0.66          & 2.17          & 90.60          & \textbf{92.74}  \\ \hline
\multirow{3}{*}{Nano distill}  & 480 x 270 & 0.98          & 0.73          & 2.09          & 88.08          & 91.23           \\
                               & 640 x 360 & 0.90          & 0.73          & 2.24          & 86.00          & 89.30           \\
                               & 960 x 540 & 0.87          & 0.70          & 2.19          & 84.73          & 86.92           \\ \hline
\multirow{3}{*}{Small}         & 480 x 270 & 0.87          & 0.68          & 2.16          & 91.08          & 91.85           \\
                               & 640 x 360 & \textbf{0.76} & \textbf{0.58} & \textbf{2.01} & 91.02          & 92.16           \\
                               & 960 x 540 & 0.81          & 0.62          & 2.08          & \textbf{92.09} & 91.86           \\ \hline
\multirow{3}{*}{Small distill} & 480 x 270 & 0.91          & 0.73          & 2.24          & 85.45          & 91.00           \\
                               & 640 x 360 & 0.84          & 0.65          & 2.16          & 85.05          & 89.68           \\
                               & 960 x 540 & 0.83          & 0.70          & 2.16          & 84.73          & 90.07           \\ \hline
\multirow{3}{*}{Medium}        & 480 x 270 & 0.84          & 0.67          & 2.15          & 91.55          & 87.44           \\
                               & 640 x 360 & 0.86          & 0.69          & 2.21          & 91.32          & 90.68           \\
                               & 960 x 540 & 0.82          & 0.63          & 2.13          & 91.23          & 91.01           \\ \hline
\multirow{3}{*}{Large}         & 480 x 270 & 0.87          & 0.70          & 2.25          & 90.85          & 91.12           \\
                               & 640 x 360 & 0.84          & 0.66          & 2.16          & 90.34          & 90.67           \\
                               & 960 x 540 & 0.81          & 0.62          & 2.14          & 91.11          & 89.61           \\ \hline
\end{tabular}
\caption{Speed measurement evaluation on BrnoCompSpeed split test C, using FP16.}
\label{tb:fp16titan}
\end{table*}
%\end{landscape}


\begin{comment}
%\begin{landscape}
\begin{table*}[h]
\centering
\begin{tabular}{@{}clcccccc@{}}
\toprule
Models &
  \begin{tabular}[c]{@{}c@{}}Input size \\ (px)\end{tabular} &
  \begin{tabular}[c]{@{}c@{}}Mean error \\ (km/h)\end{tabular} &
  \begin{tabular}[c]{@{}c@{}}Median error \\ (km/h)\end{tabular} &
  \begin{tabular}[c]{@{}c@{}}95-th percentile \\ (km/h)\end{tabular} &
  \begin{tabular}[c]{@{}c@{}}Mean precision \\ (\%)\end{tabular} &
  \begin{tabular}[c]{@{}c@{}}Mean recall \\ (\%)\end{tabular} &
  FPS \\ \midrule
\multirow{2}{*}{Nano}  & 480 x 270 & 0.86 & 0.69 & 0.69 & 88.06 & 90.34 & 47 \\
                       & 640 x 360 & 0.8  & 0.63 & 2.04 & 89.62 & 91.35 & 30 \\ \midrule
\multirow{2}{*}{Small} & 480 x 270 & 0.87 & 0.68 & 2.15 & 90.99 & 91.93 & 25 \\
                       & 640 x 360 & 0.76 & 0.58 & 2.01 & 91.02 & 91.27 & 15 \\ \bottomrule
\end{tabular}
\caption{Speed measurement evaluation on BrnoCompSpeed split test C, using FP16 and running on NVIDIA 940M.}
\label{tb:940m}
\end{table*}
\end{comment}

\begin{comment}
\begin{table*}[h]
\centering
\begin{tabular}{@{}cccccccc@{}}
\toprule
Models &
  \begin{tabular}[c]{@{}c@{}}Input size \\ (px)\end{tabular} &
  \begin{tabular}[c]{@{}c@{}}Mean error \\ (km/h)\end{tabular} &
  \begin{tabular}[c]{@{}c@{}}Median error \\ (km/h)\end{tabular} &
  \begin{tabular}[c]{@{}c@{}}95-th percentile \\ (km/h)\end{tabular} &
  \begin{tabular}[c]{@{}c@{}}Mean precision \\ (\%)\end{tabular} &
  \begin{tabular}[c]{@{}c@{}}Mean recall \\ (\%)\end{tabular} &
  FPS \\ \midrule
\multirow{3}{*}{Nano quantized}  & 480 x 270 & 0.89 & 0.69 & 2.17 & 88.40 & 87.56 & 554 \\
                                 & 640 x 360 & 0.82 & 0.64 & 2.04 & 89.20 & 89.23 & 355 \\
                                 & 960 x 540 & 0.87 & 0.69 & 2.17 & 88.40 & 89.93 & 256 \\ \midrule
\multirow{3}{*}{Small quantized} & 480 x 270 & 0.88 & 0.68 & 2.15 & 89.10 & 89.30 & 489 \\
                                 & 640 x 360 & 0.78 & 0.60 & 2.02 & 91.30 & 92.34 & 302 \\
                                 & 960 x 540 & 0.83 & 0.62 & 2.03 & 90.30 & 91.00 & 205 \\ \bottomrule
\end{tabular}
\caption{Speed measurement evaluation on BrnoCompSpeed split test C, using INT8 and running on NVIDIA RTX 2080.}
\label{tb:int8rtx}
\end{table*}
%\end{landscape}
\end{comment}

%\begin{landscape}
\begin{table*}[h]
\centering
\begin{tabular}{lcccccc}
\hline
Models &
  \begin{tabular}[c]{@{}c@{}}Input size \\ (px)\end{tabular} &
  \begin{tabular}[c]{@{}c@{}}Mean error \\ (km/h)\end{tabular} &
  \begin{tabular}[c]{@{}c@{}}Median error \\ (km/h)\end{tabular} &
  \begin{tabular}[c]{@{}c@{}}95-th percentile \\ (km/h)\end{tabular} &
  \begin{tabular}[c]{@{}c@{}}Mean precision \\ (\%)\end{tabular} &
  \begin{tabular}[c]{@{}c@{}}Mean recall \\ (\%)\end{tabular} \\ \midrule
\multirow{3}{*}{Nano}  & 480 x 270   & 0.89 & 0.69 & 2.15 & 88.05 & 91.51 \\
                       & 640 x 360   & 0.82 & 0.65 & 2.19 & 89.62 & 91.27 \\
                       & 960 x 540   & 0.87 & 0.69 & 2.14 & 90.92 & 90.13 \\ \hline
\multirow{3}{*}{Small} & 480 x 270   & 0.88 & 0.70 & 2.09 & 88.08 & 91.23 \\
                       & 640 x 360   & 0.78 & 0.60 & 2.04 & 91.02 & 91.27 \\
                       & 960 x 540   & 0.83 & 0.62 & 2.09 & 90.60 & 90.07 \\ \hline
\end{tabular}
\caption{Speed measurement evaluation on BrnoCompSpeed split test C, using INT8.}
\label{tb:int8titan}
\end{table*}
%\end{landscape}


\begin{comment}
%\begin{landscape}
\begin{table*}[h]
\centering
\begin{tabular}{@{}clcccccc@{}}
\hline
Models &
  \begin{tabular}[c]{@{}c@{}}Input size \\ (px)\end{tabular} &
  \begin{tabular}[c]{@{}c@{}}Mean error \\ (km/h)\end{tabular} &
  \begin{tabular}[c]{@{}c@{}}Median error\\  (km/h)\end{tabular} &
  \begin{tabular}[c]{@{}c@{}}95-th percentile\\ (km/h)\end{tabular} &
  \begin{tabular}[c]{@{}c@{}}Mean precision \\ (\%)\end{tabular} &
  \begin{tabular}[c]{@{}c@{}}Mean recall\\ (\%)\end{tabular} &
  FPS \\ \hline
\multirow{2}{*}{Nano}  & 480 x 270 & 0.86 & 0.69 & 0.69 & 88.06 & 90.34 & 47 \\
                       & 640 x 360 & 0.8  & 0.63 & 2.04 & 89.62 & 91.35 & 30 \\ \midrule
\multirow{2}{*}{Small} & 480 x 270 & 0.87 & 0.68 & 2.15 & 90.99 & 91.93 & 25 \\
                       & 640 x 360 & 0.76 & 0.58 & 2.01 & 91.02 & 91.27 & 15 \\ \bottomrule
\end{tabular}
\caption{Speed measurement evaluation on BrnoCompSpeed split test C, using FP16 and running on NVIDIA 940M.}
\label{tb:940m}
\end{table*}
\end{comment}


\begin{comment}
\begin{table*}[h]
\centering
\begin{tabular}{@{}cccccccc@{}}
\hline
Models &
  \begin{tabular}[c]{@{}c@{}}Input size \\ (px)\end{tabular} &
  \begin{tabular}[c]{@{}c@{}}Mean error \\ (km/h)\end{tabular} &
  \begin{tabular}[c]{@{}c@{}}Median error\\  (km/h)\end{tabular} &
  \begin{tabular}[c]{@{}c@{}}95-th percentile\\ (km/h)\end{tabular} &
  \begin{tabular}[c]{@{}c@{}}Mean precision \\ (\%)\end{tabular} &
  \begin{tabular}[c]{@{}c@{}}Mean recall\\ (\%)\end{tabular} &
  FPS \\ \hline
\multirow{3}{*}{Nano quantized}  & 480 x 270 & 0.89 & 0.69 & 2.17 & 88.40 & 87.56 & 554 \\
                                 & 640 x 360 & 0.82 & 0.64 & 2.04 & 89.20 & 89.23 & 355 \\
                                 & 960 x 540 & 0.87 & 0.69 & 2.17 & 88.40 & 89.93 & 256 \\ \midrule
\multirow{3}{*}{Small quantized} & 480 x 270 & 0.88 & 0.68 & 2.15 & 89.10 & 89.30 & 489 \\
                                 & 640 x 360 & 0.78 & 0.60 & 2.02 & 91.30 & 92.34 & 302 \\
                                 & 960 x 540 & 0.83 & 0.62 & 2.03 & 90.30 & 91.00 & 205 \\ \bottomrule
\end{tabular}
\caption{Speed measurement evaluation on BrnoCompSpeed split test C, using INT8 and running on NVIDIA RTX 2080.}
\label{tb:int8rtx}
\end{table*}
%\end{landscape}
\end{comment}


\begin{comment}
%\begin{landscape}
\begin{table*}[h]
\centering
\begin{tabular}{lccccccc}
\hline
Models &
  \begin{tabular}[c]{@{}c@{}}Input size \\ (px)\end{tabular} &
  \begin{tabular}[c]{@{}c@{}}Mean error \\ (km/h)\end{tabular} &
  \begin{tabular}[c]{@{}c@{}}Median error\\  (km/h)\end{tabular} &
  \begin{tabular}[c]{@{}c@{}}95-th percentile\\ (km/h)\end{tabular} &
  \begin{tabular}[c]{@{}c@{}}Mean precision \\ (\%)\end{tabular} &
  \begin{tabular}[c]{@{}c@{}}Mean recall\\ (\%)\end{tabular} &
  FPS \\ \hline
\multirow{3}{*}{Nano}  & 480 x 270 & 0.89 & 0.69 & 2.15 & 88.05 & 91.51 & 464 \\
                                 & 640 x 360 & 0.82 & 0.65 & 2.19 & 89.62 & 91.27 & 355 \\
                                 & 960 x 540 & 0.84 & 0.69 & 2.14 & 90.92 & 90.13 & 246 \\ \hline
\multirow{3}{*}{Small} & 480 x 270 & 0.88 & 0.70 & 2.09 & 88.08 & 91.23 & 392 \\
                                 & 640 x 360 & 0.78 & 0.60  & 2.04 & 91.02 & 91.27 & 302 \\
                                 & 960 x 540 & 0.83 & 0.62 & 2.09 & 90.60 & 90.07 & 198 \\ \hline
\end{tabular}
\caption{Speed measurement evaluation on BrnoCompSpeed split test C, using INT8 and running on NVIDIA Titan V.}
\label{tb:940m}
\end{table*}
%\end{landscape}
\end{comment}


%%JETSON

\begin{table*}[]
\begin{tabular}{p{35mm}cccccccc}
\hline
  Models &
  Data Type &
  \begin{tabular}[c]{@{}c@{}}Input size \\ (px)\end{tabular} &
  \begin{tabular}[c]{@{}c@{}}940M \\ (FPS)\end{tabular} &
  \begin{tabular}[c]{@{}c@{}}RTX 2080 \\ (FPS)\end{tabular} &
  \begin{tabular}[c]{@{}c@{}}Titan V \\ (FPS)\end{tabular} &
  \begin{tabular}[c]{@{}c@{}}TX2 \\ (FPS)\end{tabular} &
  \begin{tabular}[c]{@{}c@{}}Xavier \\ (FPS)\end{tabular} & 
  \begin{tabular}[c]{@{}c@{}}Orin \\ (FPS)\end{tabular} 
  \\ \hline
\multirow{9}{*}{Nano}          & \multirow{3}{*}{INT8} & 480 x 270 & - & 554 & 464 & - & 52 & 95 \\
                               &                       & 640 x 360 & - & 355 & 355 & - & 38 & 68 \\
                               &                       & 960 x 540 & - & 256 & 246 & - & 21 & 57 \\ 
                               & \multirow{3}{*}{F16}  & 480 x 270 & 49 & 436 & 357 & 19 & 44 & 76 \\
                               &                       & 640 x 360 & 25 & 311 & 267 & 17 & 35 & 54 \\
                               &                       & 960 x 540 & 14 & 194 & 179 & 9 & 27 & 38 \\
                               & \multirow{3}{*}{F32}  & 480 x 270 & 38 & 295 & 295 & 30 & 38 & 65 \\
                               &                       & 640 x 360 & 20 & 224 & 221 & 19 & 29 & 43 \\
                               &                       & 960 x 540 & 10 & 148 & 132 & 12 & 19 & 31 \\ \hline 
%\multirow{9}{*}{Nano distill}  & \multirow{3}{*}{INT8} & 480 x 270 & - & - & - & - & - & - \\
%                               &                       & 640 x 360 & - & - & - & - & - & - \\
%                               &                       & 960 x 540 & - & - & - & - & - & - \\
%                               & \multirow{3}{*}{F16}  & 480 x 270 & ? & 360 & 357 & 32 & 45 & 76 \\
%                               &                       & 640 x 360 & ? & 317 & 261 & 18 & 35 & 54 \\
%                               &                       & 960 x 540 & ? & 196 & 135 & ? & 31 & 39 \\
%                               & \multirow{3}{*}{F32}  & 480 x 270 & ? & 296 & 289 & 35 & 39 & 65 \\
%                               &                       & 640 x 360 & ? & 227 & 217 & 19 & 30 & 46 \\
%                               &                       & 960 x 540 & ? & 145 & 140 & ? & 19 & 30 \\ \hline 
\multirow{9}{*}{Small}         & \multirow{3}{*}{INT8} & 480 x 270 & - & 489 & 392 & - & 44 & 126 \\
                               &                       & 640 x 360 & - & 302 & 302 & - & 33 & 90 \\
                               &                       & 960 x 540 & - & 205 & 198 & - & 16 & 95 \\
                               & \multirow{3}{*}{F16}  & 480 x 270 & 23 & 448 & 354 & 15 & 44 & 58 \\
                               &                       & 640 x 360 & 14 & 243 & 205 & 8 & 36 & 39 \\
                               &                       & 960 x 540 & 6 & 145 & 139 & 5 & 18 & 24 \\
                               & \multirow{3}{*}{F32}  & 480 x 270 & 17 & 229 & 223 & 17 & 28 & 45 \\
                               &                       & 640 x 360 & 11 & 142 & 142 & 9 & 22 & 30 \\
                               &                       & 960 x 540 & 4 & 95 & 98 & 5 & 10 & 18 \\ \hline 
%\multirow{9}{*}{Small distill} & \multirow{3}{*}{INT8} & 480 x 270 & - & - & - & - & - & - \\
%                               &                       & 640 x 360 & - & - & - & - & - & - \\
%                               &                       & 960 x 540 & - & - & - & - & - & - \\
%                               & \multirow{3}{*}{F16}  & 480 x 270 & ? & 223 & 242 & 15 & 45 & 58 \\
%                               &                       & 640 x 360 & ? & 244 & 204 & ? & 38 & 38 \\
%                               &                       & 960 x 540 & ? & 144 & 170 & ? & 18 & 24 \\
%                               & \multirow{3}{*}{F32}  & 480 x 270 & ? & 226 & 219 & 18 & 27 & 46 \\
%                               &                       & 640 x 360 & ? & 143 & 143 & ? & 20 & 30 \\
%                               &                       & 960 x 540 & ? & 93 & 102 & ? & 10 & 17 \\ \hline 
\multirow{6}{*}{Medium}        & \multirow{3}{*}{F16} & 480 x 270 & 13 & 356 & 330 & 8 & 36 & 39 \\
                               &                       & 640 x 360 & 6 & 183 & 174 & 5 & 21 & 24 \\
                               &                       & 960 x 540 & 2 & 110 & 108 & 2 & 12 & 14 \\
                               & \multirow{3}{*}{F32}  & 480 x 270 & 10 & 187 & 162 & 9 & 21 & 31 \\
                               &                       & 640 x 360 & 5 & 128 & 120 & 5 & 13 & 19 \\
                               &                       & 960 x 540 & 2 & 55 & 67 & 2 & 5 & 9 \\ \hline 
\multirow{6}{*}{Large}         & \multirow{3}{*}{F16} & 480 x 270 & - & 252 & 271 & - & 28 & 29 \\
                               &                       & 640 x 360 & - & 143 & 159 & - & 17 & 18 \\
                               &                       & 960 x 540 & - & 90 & 84 & - & 9 & 10 \\
                               & \multirow{3}{*}{F32}  & 480 x 270 & - & 130 & 125 & - & 15 & 21 \\
                               &                       & 640 x 360 & - & 95 & 95 & - & 8 & 14 \\
                               &                       & 960 x 540 & - & 40 & 50 & - & 3 & 7 \\ \hline 
\end{tabular}
\caption{Speed benchmark across various devices for different input sizes and data types.}
\label{tb:fp16titan}
\end{table*}



\begin{table*}[]
\begin{tabular}{p{35mm}cccc}
\hline
  Models &
  \begin{tabular}[c]{@{}c@{}}Input size \\ (px)\end{tabular} &
  \begin{tabular}[c]{@{}c@{}}Low Traffic Titan V\\ Session 4 (FPS)\end{tabular} &
  \begin{tabular}[c]{@{}c@{}}Medium Traffic Titan V\\ Session 6 (FPS)\end{tabular} &
  \begin{tabular}[c]{@{}c@{}}Dense Traffic Titan V\\ Session 5 (FPS)\end{tabular} 
  \\ \hline
\multirow{3}{*}{Nano}          & 480 x 270 & 353 & 305 & 319 \\
                               & 640 x 360 & 297 & 246 & 258 \\
                               & 960 x 540 & 185 & 166 & 175 \\ \hline 
\multirow{3}{*}{Small}         & 480 x 270 & 351 & 288 & 313 \\
                               & 640 x 360 & 260 & 220 & 239 \\
                               & 960 x 540 & 156 & 129 & 145 \\ \hline 
\multirow{3}{*}{Medium}        & 480 x 270 & 288 & 249 & 262 \\
                               & 640 x 360 & 197 & 178 & 184 \\
                               & 960 x 540 & 114 & 98 & 108 \\ \hline 
\multirow{3}{*}{Large}         & 480 x 270 & 249 & 230 & 229 \\
                               & 640 x 360 & 168 & 147 & 159 \\
                               & 960 x 540 & 89 & 86 & 87 \\ \hline 
\end{tabular}
\caption{Speed benchmark for different traffic situations.}
\label{tb:situations}
\end{table*}
